# Supplementary material for: SWIFT: Sliding Window Reconstruction for Few-Shot Training-Free Generated Video Attribution
Source: arXiv:2603.08536 source file (2026-03-21)
Supplement: Supplementary file 1 [file X_suppl.tex]

\clearpage
\setcounter{page}{1}
\maketitlesupplementary

\section{Performance Degradation of AEDR}
Although AEDR~\cite{AEDR} performs excellently in image modality, its accuracy significantly drops when transferred to video modality. The cause of this phenomenon lies in the introduction of complex temporal characteristics in video modality, which disrupts the core assumption of AEDR: the loss ratio for belonging samples in two consecutive reconstructions should be close to 1, while the ratio for non-belonging samples is significantly greater than 1. Specifically, video VAEs need to simultaneously account for both spatial and temporal dimensions, and their latent space exhibits a high degree of temporal coupling—motion information and dependencies between adjacent frames are compressed and shared within the latent space, which considerably increases the difficulty of reconstruction. Therefore, this complex temporal coupling and cross-frame dependencies lead to a systematic increase in the loss of the first reconstruction, causing the loss ratio for belonging videos to deviate from 1 as well (see \cref{AEDR-Dis}). The failure of AEDR stems from its focus solely on spatial consistency during reconstruction, while videos also entail temporal consistency.

\begin{figure}[t]
\centering
\includegraphics[width=0.98\linewidth]{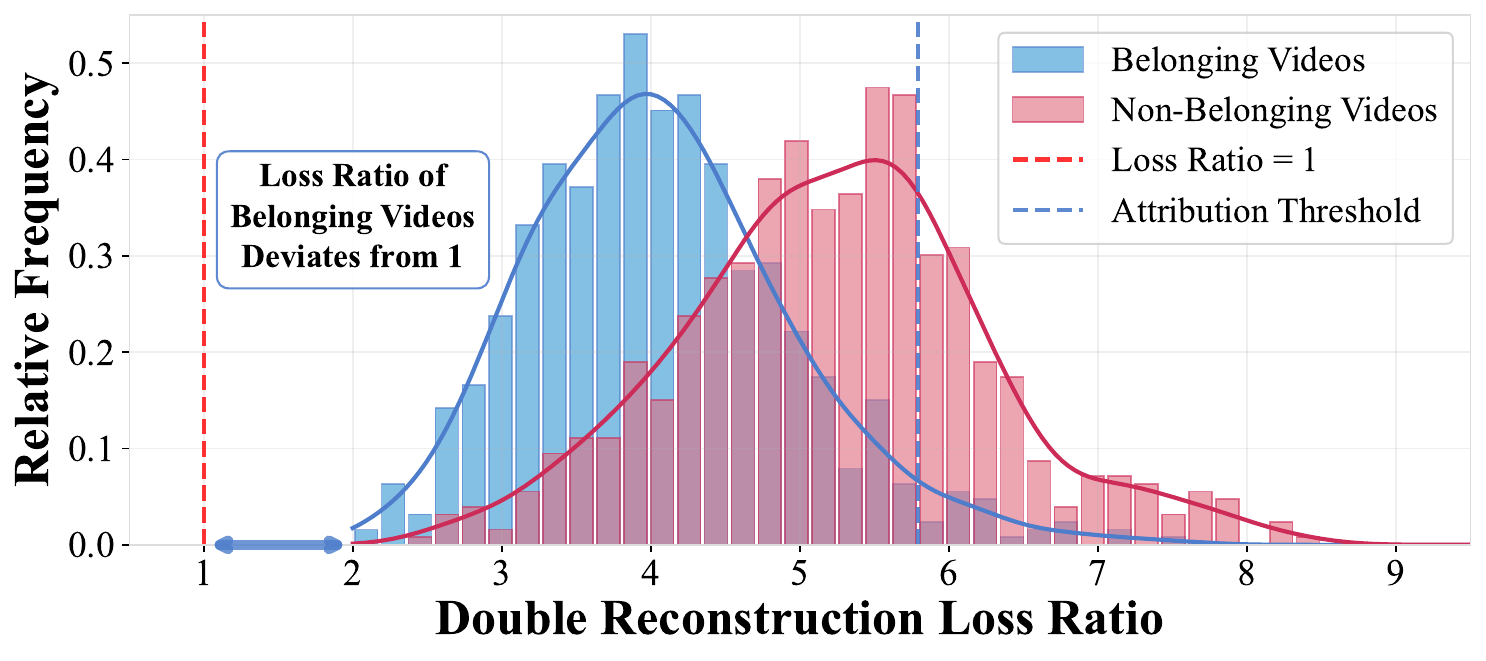}
\vspace{-0.3cm}
\caption{Performance of AEDR in video modality (belonging model: HunyuanVideo~\cite{HYV}, non-belonging model: EasyAnimate~\cite{EA}). The loss ratio for attributed videos deviates from 1, and the increased attribution threshold (Threshold=5.79) results in non-belonging videos being incorrectly classified as belonging.}
\label{AEDR-Dis}
\vspace{-0.3cm} 
\end{figure}

\section{More Details of the S-Video}
Our dataset (S-Video) comprises a total of 4,000 videos, with 500 real videos and 3,500 generated videos. The real videos were randomly sampled from the OpenVidHD~\cite{OpenVid}, while the generated videos were produced using 700 randomly selected prompts from OpenVidHD and five different generative models. \cref{Generated-Sample} presents samples of videos generated using the same prompts across the five models. \cref{Real-Sample} displays samples of real videos, and \cref{Prompt-Dataset} provides a list of the prompts used in the generation process.

\begin{figure*}[t]
\centering

\begin{subfigure}[b]{0.96\linewidth}
    \centering
    \includegraphics[width=\linewidth]{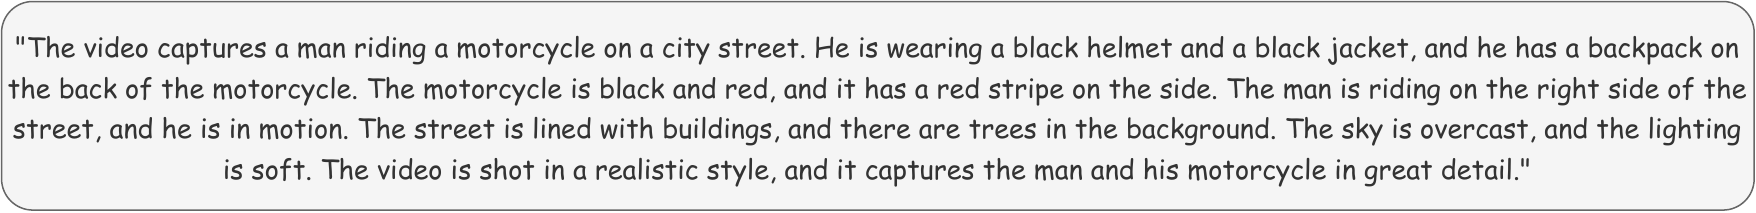}
    \caption{The following five video samples are generated using this prompt.}
\end{subfigure}

\begin{subfigure}[b]{0.96\linewidth}
    \centering
    \includegraphics[width=\linewidth]{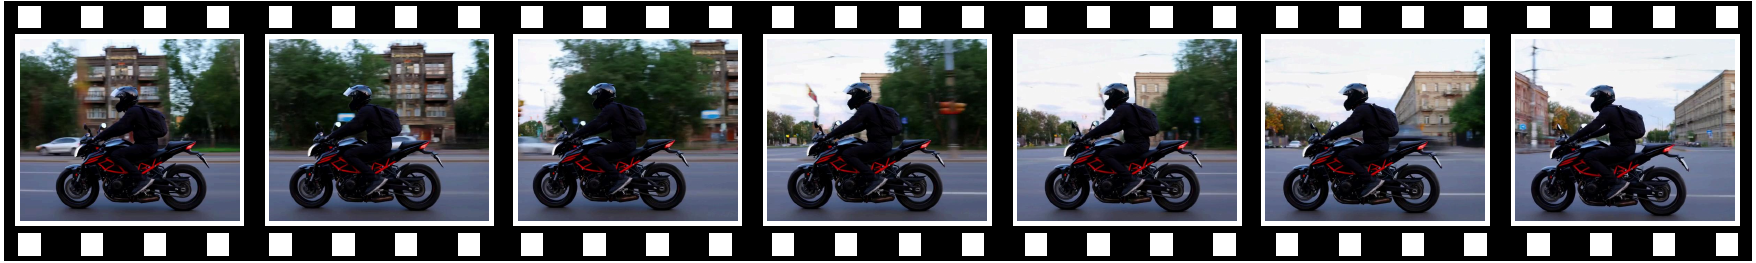}
    \caption{A sample video generated by HunyuanVideo~\cite{HYV}.}
\end{subfigure}

\begin{subfigure}[b]{0.96\linewidth}
    \centering
    \includegraphics[width=\linewidth]{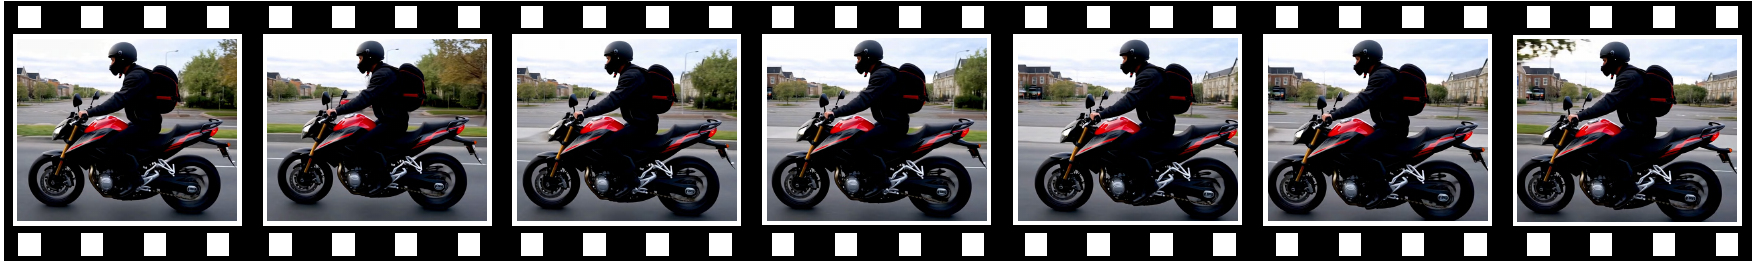}
    \caption{A sample video generated by Wan2.1~\cite{Wan2.1}.}
\end{subfigure}

\begin{subfigure}[b]{0.96\linewidth}
    \centering
    \includegraphics[width=\linewidth]{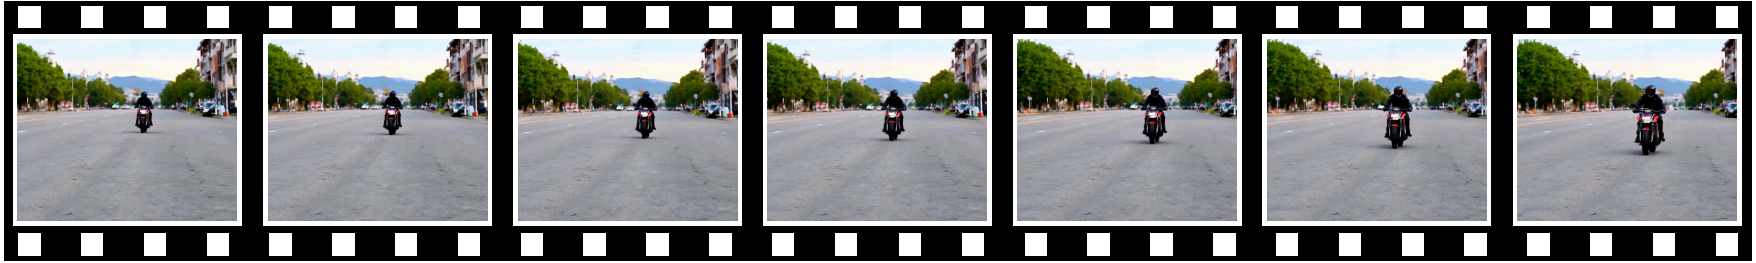}
    \caption{A sample video generated by LTX-Video~\cite{LTX}.}
\end{subfigure}

\begin{subfigure}[b]{0.96\linewidth}
    \centering
    \includegraphics[width=\linewidth]{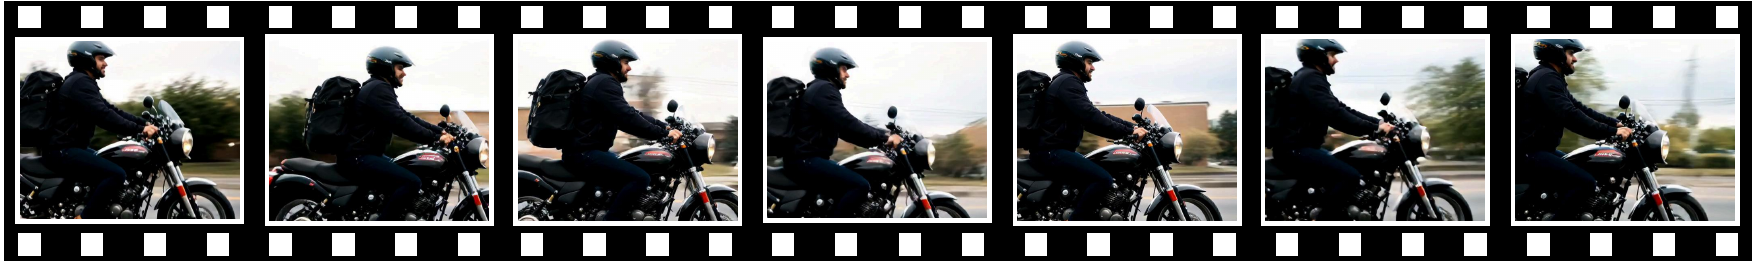}
    \caption{A sample video generated by EasyAnimate~\cite{EA}.}
\end{subfigure}

\begin{subfigure}[b]{0.96\linewidth}
    \centering
    \includegraphics[width=\linewidth]{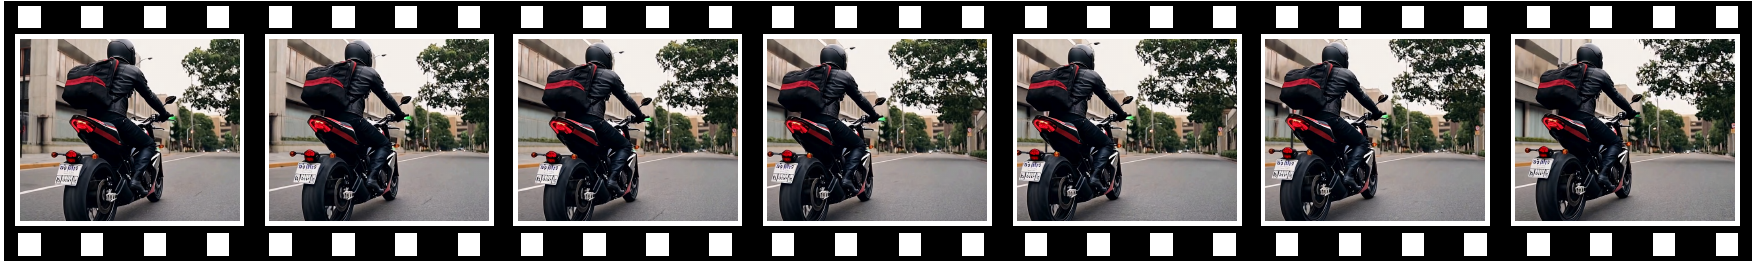}
    \caption{A sample video generated by Wan2.2~\cite{Wan2.1}.}
\end{subfigure}
\vspace{-0.3cm}
\caption{Video samples generated by the five models using the same prompt.}
\label{Generated-Sample}
\end{figure*}

\begin{figure*}[] 
\centering 
\includegraphics[width=0.96\linewidth]{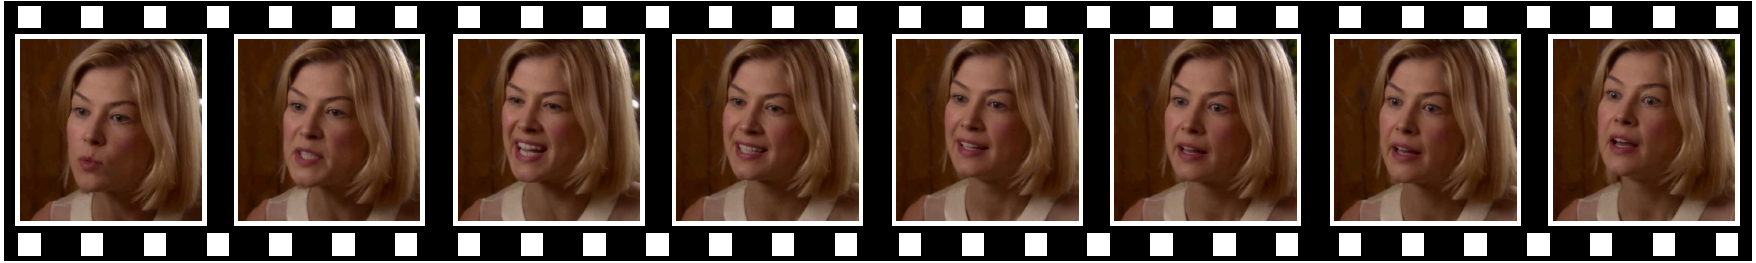} 
\caption{A real video sample randomly drawn from the OpenVidHD-1M~\cite{OpenVid}.} 
\label{Real-Sample}
\end{figure*}

\section{Evaluation Metrics}
\label{Acc}
In this paper, we utilize accuracy (Acc) as the metric to evaluate the attribution performance of the algorithm. The goal of SWIFT is to determine whether a given video belongs to the target model, which involves binary classification (belonging vs. non-belonging). The evaluation takes into account four key outcomes: True Positives (TP), where belonging videos are correctly identified; False Positives (FP), where non-belonging videos are misclassified as belonging; False Negatives (FN), where belonging videos are mistakenly identified as non-belonging; and True Negatives (TN), where non-belonging videos are correctly identified.

% \section{Selection of KDE Parameters}
% \label{Selection of KDE Parameters}
% To assess the impact of bandwidth and kernel function on attribution accuracy, we used the EA~\cite{EA} as the target model and tested it across all videos in the dataset. We tested two commonly used bandwidth selection methods: Scott's method and Silverman’s method, alongside three commonly used kernel functions: Gaussian kernel, Uniform kernel, and Epanechnikov kernel. The results, shown in \cref{KDE}, indicate that the choice of bandwidth and kernel function has a negligible effect on the final attribution accuracy, with fluctuations not exceeding 0.5\%. Therefore, we selected the combination of Scott's method for bandwidth and the Gaussian kernel as the default configuration for this paper, as it provided the best overall performance.

\begin{table}[t]
\centering
\caption{Examples of text prompts used to create the S-Video.}
\begin{tabular}{p{0.95\columnwidth}}
\toprule
\textbf{Prompt Examples} \\ 
\midrule
\addlinespace[0.3em]
The video features a young man with a black cap and a black t-shirt, standing in a skate park. He is smiling and looking directly at the camera. The skate park is filled with ramps and rails, and the ground is covered in a light blue paint. The background is slightly blurred, but it appears to be a cloudy day. The man's casual attire and the skate park setting suggest that this is a casual. \\
\addlinespace[0.3em]
\midrule
\addlinespace[0.3em]
In the video, a person is seen preparing a salad in a white bowl placed on a wooden table. The salad consists of various ingredients such as lettuce, tomatoes, beans, and avocado. The person is using a spoon to mix the ingredients together. The table also has a pen and a bowl of chips. The overall style of the video is casual and homey, capturing a simple yet enjoyable cooking moment. \\
\addlinespace[0.3em]
\midrule
\addlinespace[0.3em]
The video features a woman with blonde hair and blue eyes, wearing a black top and gold earrings. She is making a peace sign with her right hand and has her mouth open as if she is speaking or singing. The background shows a staircase with a white railing and a white wall. The style of the video is casual and informal, with a focus on the woman's expression and gesture. \\
\addlinespace[0.3em]
\midrule
\addlinespace[0.3em]
In the video, a man and a woman are seated at a dining table in a kitchen, enjoying a meal together. The man is wearing a yellow and black plaid hoodie, while the woman is dressed in a pink hoodie. They are both eating from white bowls filled with a green and yellow dish, possibly a soup or stew. The kitchen is equipped with modern appliances, including a microwave and an oven. \\
\addlinespace[0.3em]
% \midrule
% \addlinespace[0.3em]
% The video features a young man in a dark blue soccer jersey with a logo on the left chest and the word ``Nike" on the right chest. He is standing on a grassy field with trees in the background. The man is looking to his left with a slight smile on his face. The style of the video is a close-up shot with a shallow depth of field, focusing on the man's face and upper body. The lighting is natural, suggesting it is daytime. The man's attire and the field setting suggest that he is a soccer player. 
\bottomrule
\end{tabular}
\label{Prompt-Dataset}
\vspace{-0.5cm}
\end{table}

% \begin{table}[]
% \centering
% \caption{Impact of bandwidth and kernel function on accuracy.}
% \resizebox{0.78\columnwidth}{!}{%
% \begin{tabular}{c|c|c}
% \toprule
% Bandwidth & Kernel Function & Avg Acc \\
% \midrule
% \multirow{3}{*}{Scott} & Gaussian & \textbf{97.80\%} \\
%  & Uniform & 97.40\% \\
%  & Epanechnikov & 97.40\% \\
% \midrule
% \multirow{3}{*}{Silverman} & Gaussian & \textbf{97.80\%} \\
%  & Uniform & 97.30\% \\
%  & Epanechnikov & 97.40\% \\
% \bottomrule
% \end{tabular}%
% }
% \label{KDE}
% \end{table}

\begin{figure*}[t]
    \centering
    \begin{subfigure}[b]{0.43\linewidth}
        \centering
        \includegraphics[width=\linewidth]{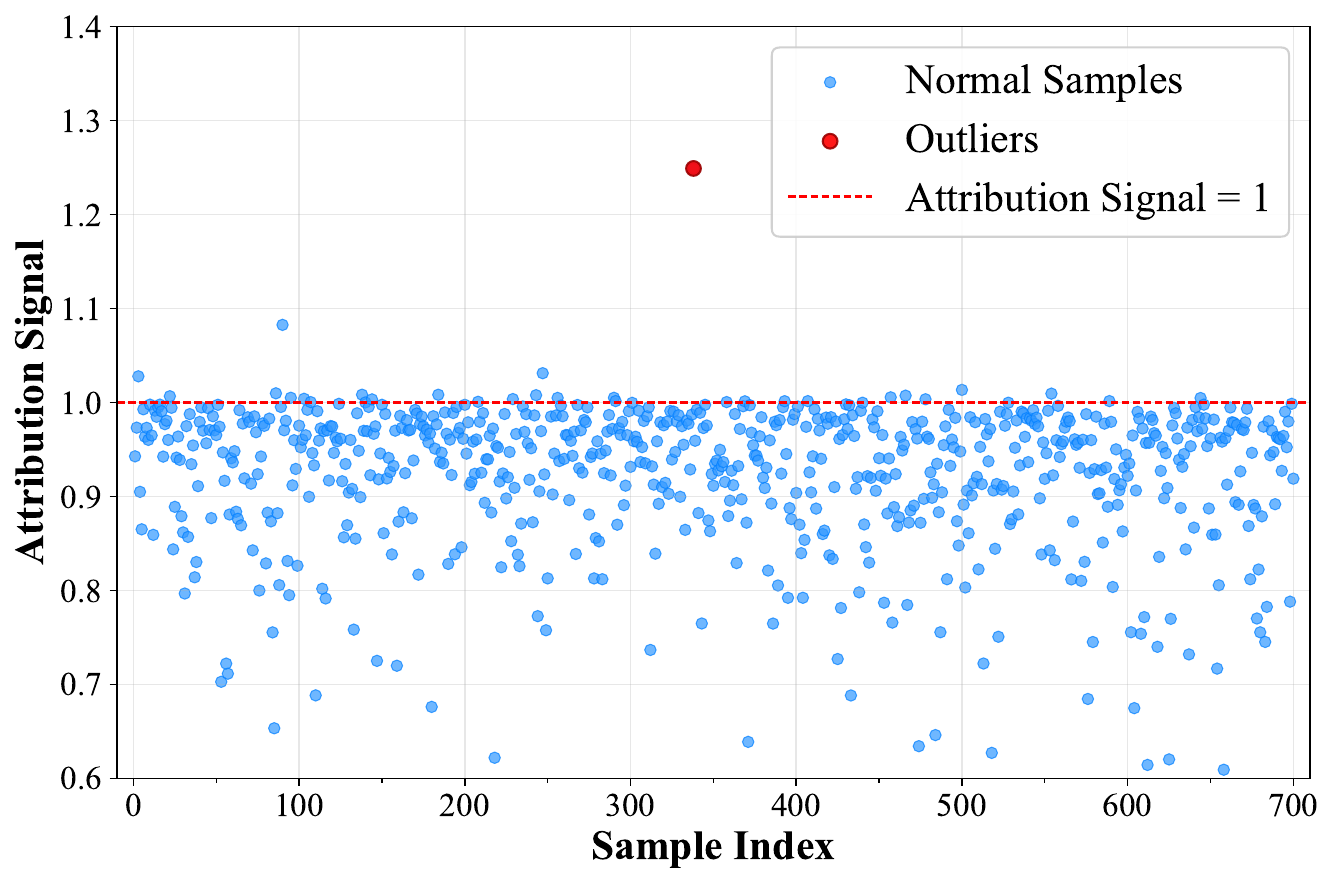}
        \caption{Attribution signal distribution of HYV~\cite{HYV}.}
        \label{Dis-1}
    \end{subfigure}
    \begin{subfigure}[b]{0.43\linewidth}
        \centering
        \includegraphics[width=\linewidth]{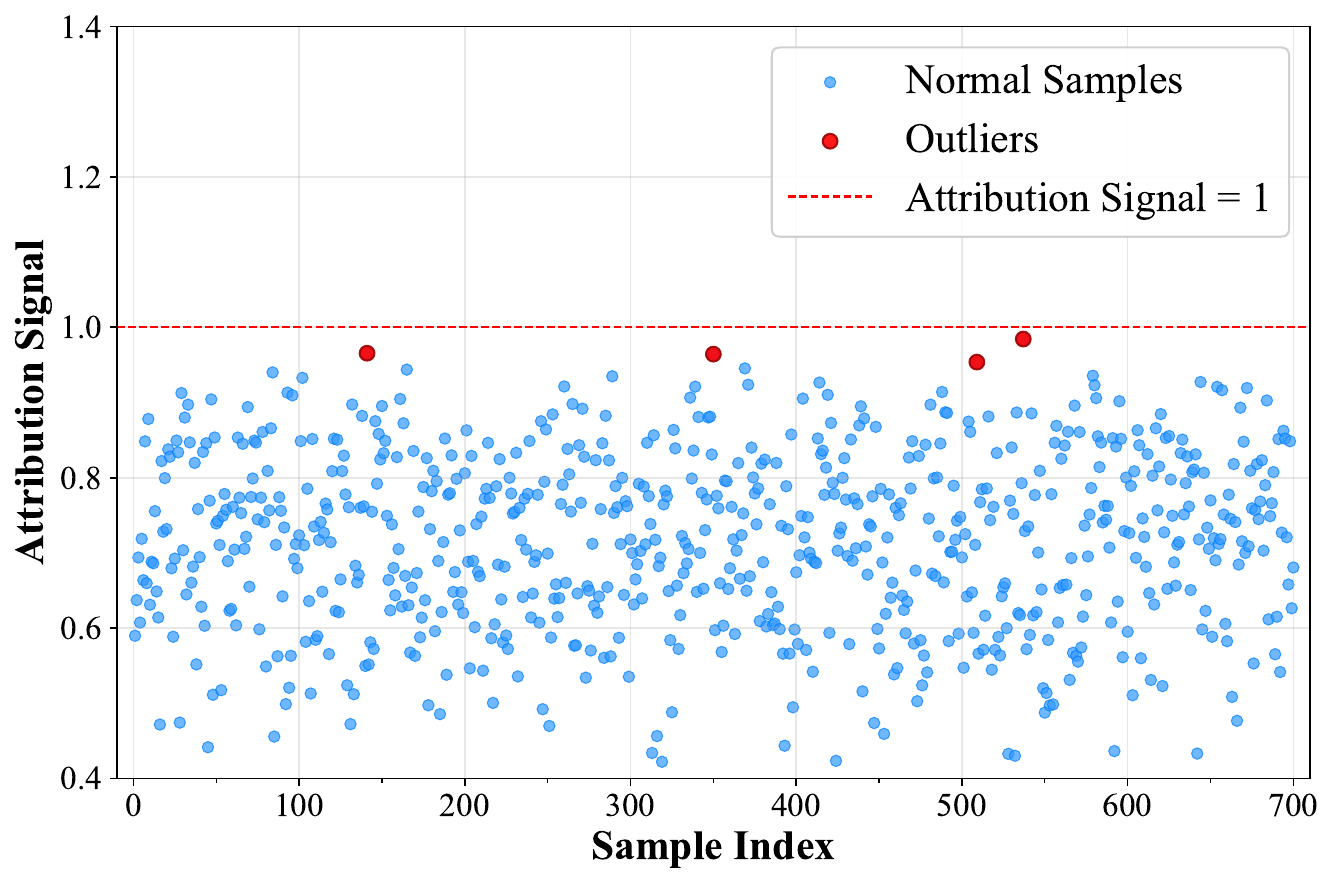}
        \caption{Attribution signal distribution of Wan2.1~\cite{Wan2.1}.}
        \label{Dis-2}
    \end{subfigure}

    \begin{subfigure}[b]{0.43\linewidth}
        \centering
        \includegraphics[width=\linewidth]{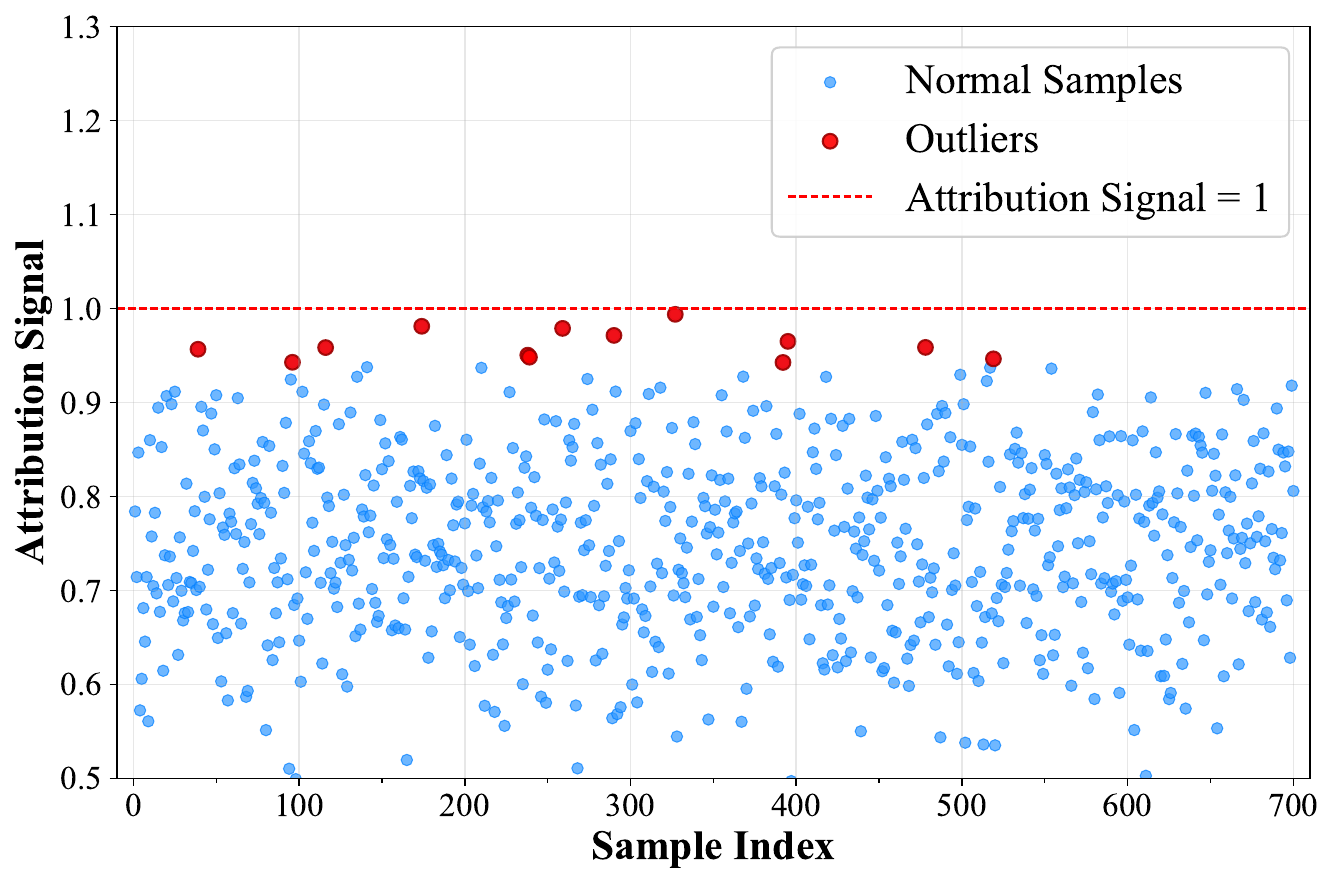}
        \caption{Attribution signal distribution of LTX~\cite{LTX}.}
        \label{Dis-3}
    \end{subfigure}
    \begin{subfigure}[b]{0.43\linewidth}
        \centering
        \includegraphics[width=\linewidth]{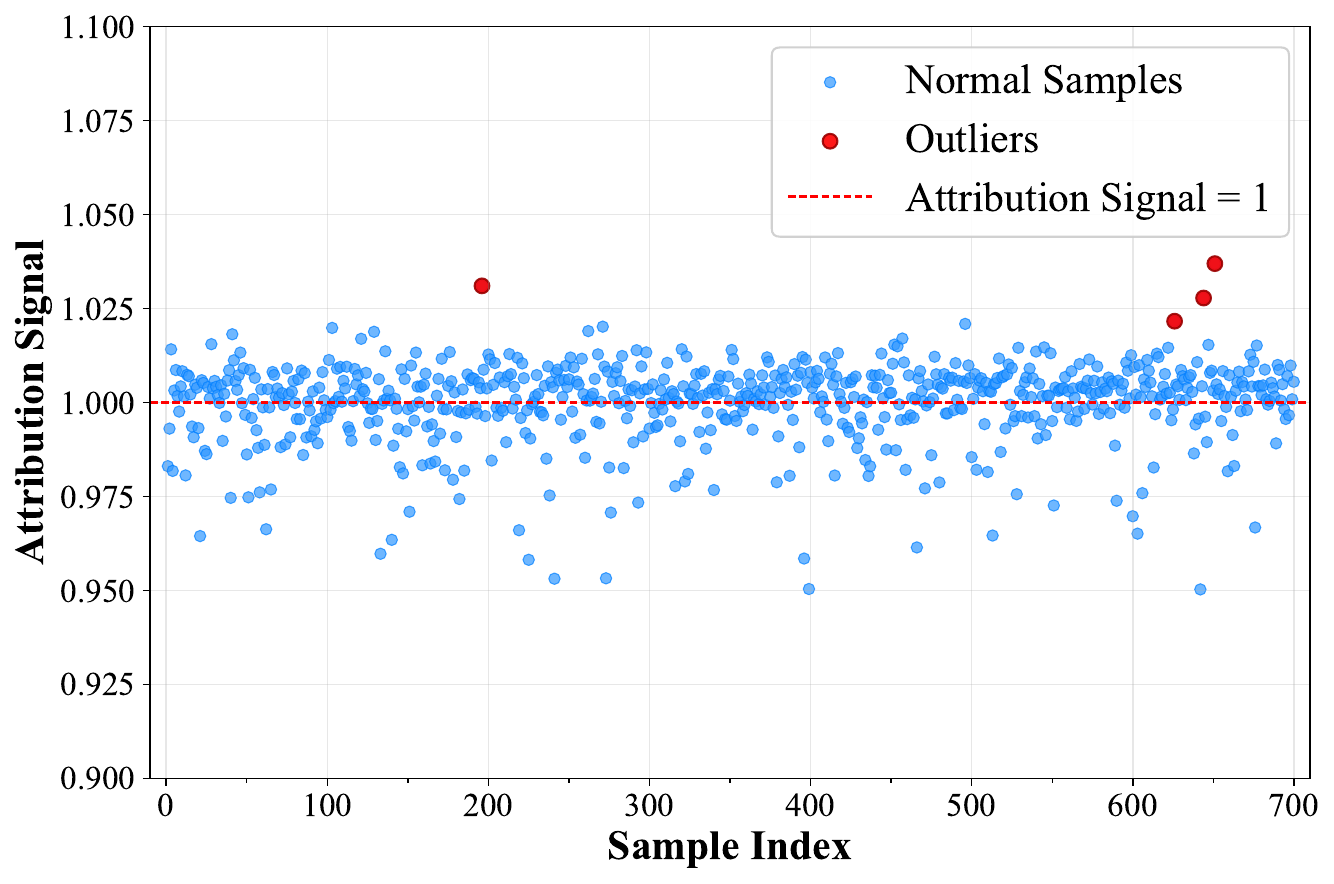}
        \caption{Attribution signal distribution of EA~\cite{EA}.}
        \label{Dis-4}
    \end{subfigure}
    
    \begin{subfigure}[b]{0.43\linewidth}
        \centering
        \includegraphics[width=\linewidth]{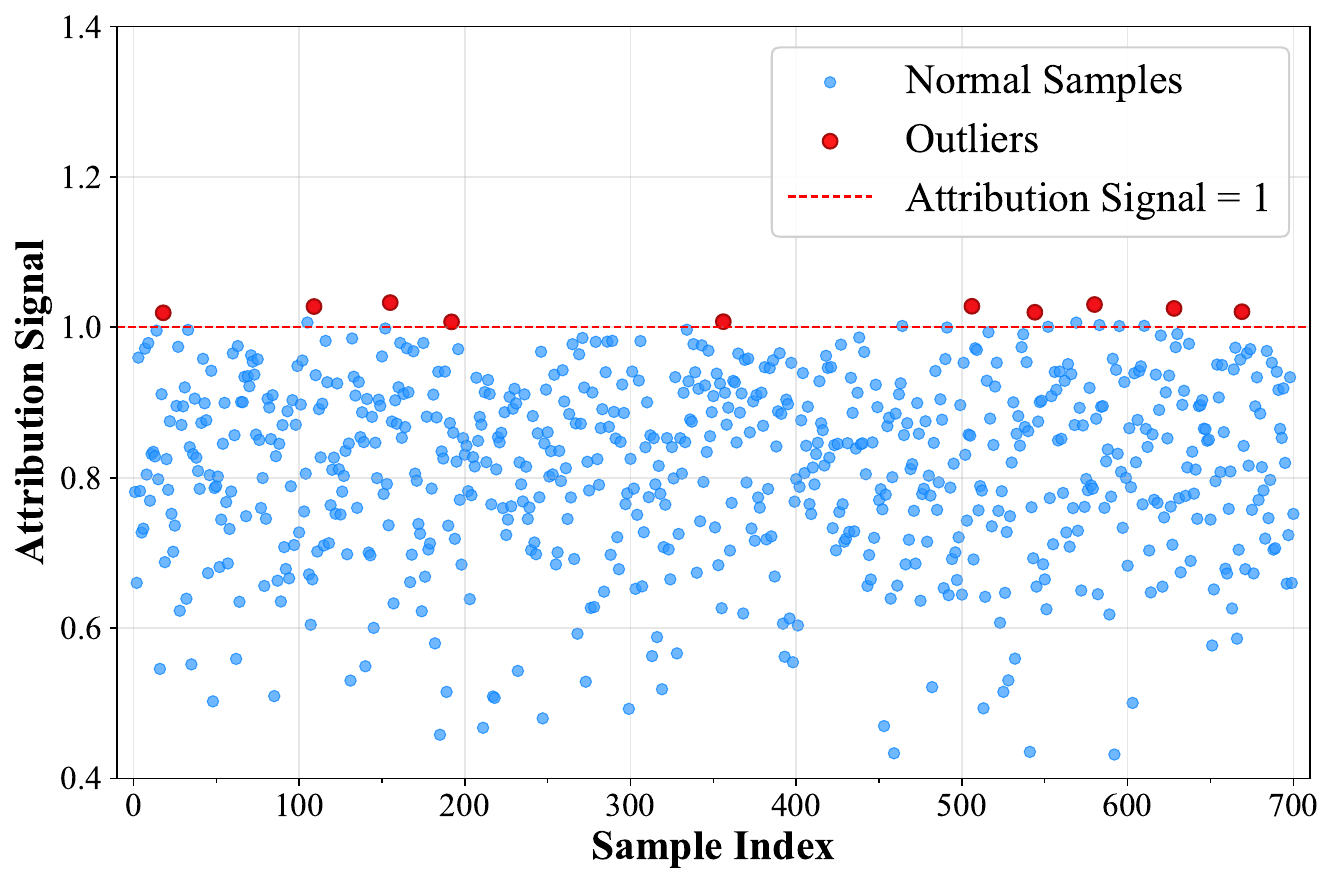}
        \caption{Attribution signal distribution of Wan2.2~\cite{Wan2.1}.}
        \label{Dis-5}
    \end{subfigure}
    \vspace{-0.2cm}
    \caption{The distribution of attribution signals and outliers for the five models mentioned in this paper.}
    \label{Distribution}
\vspace{-0.5cm}
\end{figure*}

\section{Distribution of Attribution Signal}
\label{Distribution of Attribution Signal}
Due to the variations in model architecture and training data, the distribution of the attribution signal $t$ in the five video generation models discussed in this paper exhibits significant differences. As a result, we determined specific threshold values for each model. By testing on the belonging videos for each model, the distribution of the attribution signal $t$ for each model is shown in \cref{Distribution}. It is observed that the attribution signals for the HYV~\cite{HYV}, Wan2.1~\cite{Wan2.1}, EA~\cite{EA}, and Wan2.2~\cite{Wan2.1} are relatively dispersed, with the majority of the attribution signals in the belonging videos for these four models being less than 1. This is the fundamental reason why the HYV~\cite{HYV}, EA~\cite{EA}, and Wan2.2~\cite{Wan2.1} are capable of achieving zero-shot attribution.

In contrast, the attribution signal distribution for LTX~\cite{LTX} is highly concentrated, roughly symmetrically around 1, which provides an intuitive explanation for its inferior attribution performance compared to the aforementioned models. Furthermore, we observed that each model's belonging videos contain a small number of outliers (represented as red dots in \cref{Distribution}), which can be attributed to the inherent diversity in the generated videos. To address this issue, we employed Kernel Density Estimation~\cite{KDE}, a non-parametric method that makes no assumptions about the underlying distribution and is inherently robust to outliers.

\section{Verification of Theoretical Analysis}
Our theoretical analysis (see Section 3.2) aims to ``maximize the reconstruction discrepancy," i.e., maximize corruption (can be quantified by the MSE Loss). An intuitive and expedited strategy is to select $W_{N-1}$ as the corrupted window; for the other 4 models in the paper (excluding LTX~\cite{LTX}), $W_3$ aligns with the analysis ($N=4$). However, LTX deviates from this intuition due to its unique decoder with a denoising step. The results presented in \cref{Corrupted_levels} show that selecting $W_3$ causes the greatest corruption in LTX, thus adhering to the corruption-maximizing theory.

\begin{table}[t]
\centering
\vspace{-0.3cm}
\caption{Corrupted levels under different windows (MSE Loss).}
\vspace{-0.3cm}
\setlength{\aboverulesep}{1.5pt}
\setlength{\belowrulesep}{1.5pt}

\setlength{\tabcolsep}{4pt} 
\resizebox{\columnwidth}{!}{%
\begin{tabular}{cccc>{\columncolor{gray!25}}cccccc}
\toprule
Window & $W_0$ & $W_1$ & $W_2$ & $W_3$ & $W_4$ & $W_5$ & $W_6$ & $W_7$ & $W_8$ \\
\midrule
HYV($\times 10^{-4}$) & 5.413 & 6.592 & 6.574 & \textbf{6.674} & 5.442 & - & - & - & - \\
LTX($\times 10^{-3}$) & 1.072 & 1.081 & 1.081 & \textbf{1.087} & 1.082 & 1.084 & 1.081 & 1.077 & 1.060 \\
\bottomrule
\end{tabular}%
}
\label{Corrupted_levels}
\end{table}
